# Supplementary material for: Energy Minimization of Discrete Protein Titration State Models Using Graph Theory
Source: arXiv:1507.07021 ancillary file (2016-04-17)
Supplement: Supplementary file 1 [file supporting.pdf]

# Supporting Information for Publication

## "Energy Minimization of Discrete Protein Titration State Models Using Graph Theory"

Emilie Purvine,[*,†] Kyle Monson,[*,†] Elizabeth Jurrus,[*,†] Keith Star,[*,†] and Nathan A. Baker[*,‡]

*Computational and Statistical Analytics Division, Pacific Northwest National Laboratory, and Advanced Computing, Mathematics, and Data Division, Pacific Northwest National Laboratory; Division of Applied Mathematics, Brown University*

E-mail: emilie.purvine@pnnl.gov; kyle.monson@pnnl.gov; elizabeth.jurrus@pnnl.gov; keith@pnnl.gov; nathan.baker@pnnl.gov

# Graph theory background

In order to describe the minimization algorithm, we will need some terminology from graph theory.[1] Let $G = (V, E)$ be a *(simple) graph* where $V$ is the set of *vertices* and $E \subseteq V \times V$ is the set of *edges*. We note here that though the graph is denoted by $G$, and the edge set is denoted by $E$ they have no traditional relationship to our energy functions denoted by $G$, $E_i$, and $E_{ij}$. It is merely an unfortunate coincidence in convention that graphs, edges, and energy are written using $G$ and $E$. We say that $G$ is a *directed graph* if $[v, w] \in E$ does not imply that $[w, v] \in E$, i.e., edges have a starting vertex and ending vertex. Otherwise

*To whom correspondence should be addressed

†Computational and Statistical Analytics Division, Pacific Northwest National Laboratory

‡Advanced Computing, Mathematics, and Data Division, Pacific Northwest National Laboratory; Division of Applied Mathematics, Brown University

$G$ is *undirected*, and we will write edges as pairs $(v, w) \in E$ where order does not matter. For directed graphs, we will write edges in square brackets, $[v, w] \in E$, and maintain that the order of the vertices is important. If, in addition to $V$ and $E$, we have a function $w : E \to \mathbb{R}$ then we say that $G$ is *edge weighted*, and $w$ is the *weight function* on the edges. We also define vertex weights with weight function $g : V \to \mathbb{R}$. In addition to this generic graph terminology, we must also define flows and cuts in networks. Let $G = (V, E)$ be a directed graph, $c$ be an edge weight function called the *capacity* function, and $s, t \in V$ be two distinguished vertices, called the *source* and *sink*, respectively, so that all edges at $s$ are leaving $s$ and all edges at $t$ are arriving. Then the tuple $N = (G, s, t, c)$ is a *network*. A function $f : E \to \mathbb{R}$ is called a *flow* if it satisfies:

**(F1)** for all $v \in V \setminus \{s, t\}$, the sum of the flow values on all edges coming in to $v$ must equal the sum of the flow values on edges leaving $v$

$$\sum_{u:[u,v]\in E} f([u, v]) = \sum_{w:[v,w]\in E} f([v, w]),$$

**(F2)** for all $e \in E$, $f(e) \leq c(e)$; i.e., the flow is at most the capacity.

The *flow value* is equal to the sum of the flow values on edges leaving $s$ (which is equal to the sum of the flow values on edges arriving at $t$). A partition of the vertices into two sets $V = S \cup T$ such that $s \in S$ and $t \in T$ is called a *cut* in the network. The *cut capacity* is equal to the sum of the capacities of all the edges whose starting vertex is in $S$ and ending vertex is in $T$. The minimum cut in a network can be found through the max-flow/min-cut theorem of Ford and Fulkerson which states: given a network $N = (G, s, t, c)$, the maximum flow value is equal to the minimum cut capacity.[2] Several algorithms are available to find a maximum flow;[2–5] given a maximum flow, one can perform a depth-first search on the residual network to find the $S$ and $T$ partition for the minimum cut. See Figure S1 for an example of a maximum flow and minimum cut.

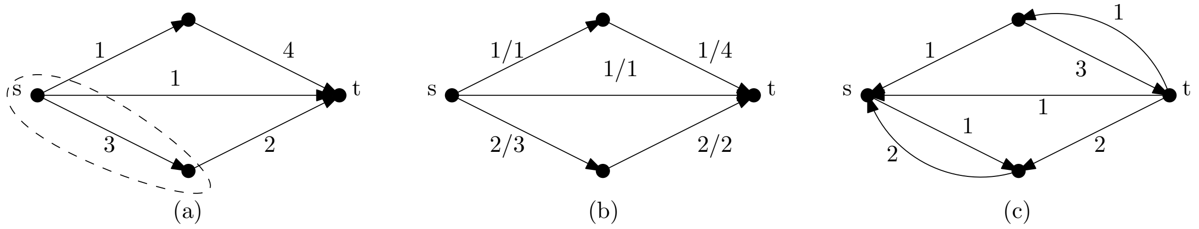


Figure S1: (a) A network with capacity function on the edges, and the minimum cut set $S$ identified by the dashed oval. (b) The same network with maximum flow on the edges, edge labels are of the form “flow/capacity”. (c) The residual network from the maximum flow in (b). Edges in the forward direction are weighted by capacity minus flow, and in the backwards direction they are weighted by the flow.

A function, $E_{ij}$ is *submodular* if

$$E_{ij}(0,0) + E_{ij}(1,1) \leq E_{ij}(1,0) + E_{ij}(0,1), \tag{1}$$

for all $1 \leq i, j \leq N$. However, we cannot assume that this is the case in general for the energy functions involved in titration state calculations.

## Energy graph construction

Each amino acid will be represented by two vertices, one for each titration state:

$$\begin{aligned} V &= \{\text{amino acid } i \text{ in deprotonated state}\}_{i=1}^{N} \cup \{\text{amino acid } i \text{ in protonated state}\}_{i=1}^{N} \\ &= \{\langle i, 0\rangle, \langle i, 1\rangle\}_{i=1}^{N}. \end{aligned}$$

Our graph is then $G = (V, E, g, w)$, with vertex weights

$$\begin{aligned} g : V &\longrightarrow \mathbb{R} \\ \langle i, b\rangle &\longmapsto E_i(b), \end{aligned}$$

and edge weights

$$w : E \longrightarrow \mathbb{R}$$

$$\langle \langle i, b_i \rangle, \langle j, b_j \rangle \rangle \longmapsto E_{ij}(b_i, b_j).$$

See Figure S2 for an example energy graph with two amino acids, $A$ and $B$.

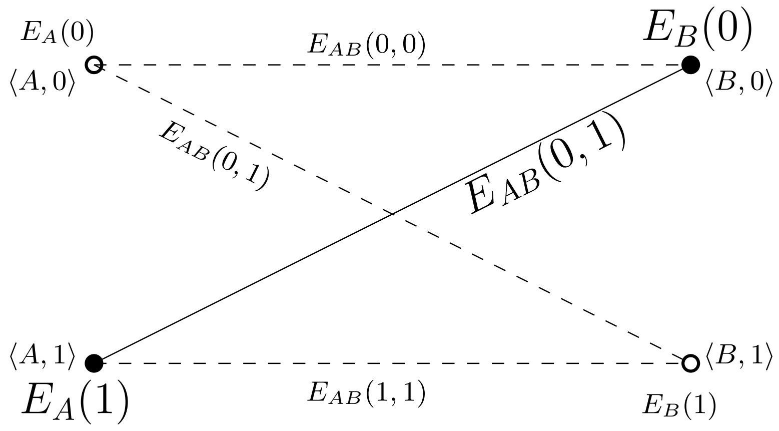


Figure S2: Energy graph for two amino acids, $A$ and $B$. To calculate the energy for the state with $A$ protonated and $B$ deprotonated, we discard vertices $\langle A, 0 \rangle$ and $\langle B, 1 \rangle$, and their associated edges as indicated by the unfilled circles and dashed edges. We then sum the remaining edge and vertex weights.

The resulting graph is an abstraction of the protein energy function wherein assigning a protonation state to the protein consists of discarding one vertex (and all edges associated with that vertex) from each pair of vertices that correspond to a single amino acid. For example, if we have amino acids $A$ and $B$, as in Figure S2, and we wish to calculate the energy for the protonation state $\langle 1, 0 \rangle$, we discard vertices $\langle A, 0 \rangle$ and $\langle B, 1 \rangle$.

The resulting graph can be simplified into *normal form* through a procedure that ensures we never change the energy of any protonation state $P \in \mathcal{P}$. Given a pair of amino acids, $i, j$, and a label $\ell \in \{0, 1\}$, consider the two edges between $\langle i, \ell \rangle$ and amino acid $j$: $e_1 = (\langle i, \ell \rangle, \langle j, 0 \rangle)$, and $e_2 = (\langle i, \ell \rangle, \langle j, 1 \rangle)$. If we replace the edge and vertex weights with new

functions $w'$ and $g'$ given by

$$w'_{i,j,\ell,d}(e) = \begin{cases} w(e) - d & \text{if } e = e_1 \text{ or } e_2 \\ w(e) & \text{otherwise} \end{cases} \qquad g'_{i,j,\ell,d}(v) = \begin{cases} g(v) + d & \text{if } v = \langle i, \ell \rangle \\ g(v) & \text{otherwise} \end{cases}$$

for some $d \in \mathbb{R}$, then we do not change the energy of any protein configurations.

Since the weights on other edges and vertices are unchanged, it is sufficient to show that this procedure does not change the energy of a protonation state for the $i$ and $j$ amino acids when amino acid $i$ is restricted to the state $\ell$. If amino acid $j$ is protonated, then we discard vertex $\langle j, 0 \rangle$ and are left with $\langle i, \ell \rangle$ and $\langle j, 1 \rangle$. Our configuration energy will then be

$$\begin{aligned} &g'_{i,j,\ell,d}(\langle i, \ell \rangle) + g'_{i,j,\ell,d}(\langle j, 1 \rangle) + w'_{i,j,\ell,d}(\langle i, \ell \rangle, \langle j, 1 \rangle) \\ &\qquad = \Big(g(\langle i, \ell \rangle) + d\Big) + g(\langle j, 1 \rangle) + \Big(w(\langle i, \ell \rangle, \langle j, 1 \rangle) - d\Big) \\ &\qquad = g(\langle i, \ell \rangle) + g(\langle j, 1 \rangle) + w(\langle i, \ell \rangle, \langle j, 1 \rangle). \end{aligned}$$

If amino acid $j$ is deprotonated, then we replace $\langle j, 1 \rangle$ with $\langle j, 0 \rangle$ and obtain the same cancellation and final energy. In order to ensure that all edge weights are non-negative and to maximize the number of edges with zero weight, we choose $d := \min\{w(e_1), w(e_2)\}$. With this choice, whichever of the two edges had the minimum weight will now have zero weight, and the weight of the other edge is ensured to be non-negative. We repeat this procedure for all ordered pairs of amino acids $[i, j]$ and all labels $\ell \in \{0, 1\}$.

After the edge re-weighting, we re-weight amino acid vertices following a similar procedure. Here we observe that the overall energy of any protonation state is unaffected by subtracting some value $a$ from the vertex weights on $\langle i, 0 \rangle$ and $\langle i, 1 \rangle$ and then adding $a$ to a universal constant $C$, to be included in the sum of edge and vertex weights when calculating the protonation state energy. Notice that doing this procedure in a different order could produce an alternate normal form energy graph; however, the overall energy function is not affected by the order of the procedures. See Figure S3 for an example of the normal form

procedure.

## Multi-state energy graph construction

The energy graph for one HIS and one non-HIS residue, prior to separating HIS into $HIS_\epsilon$ and $HIS_\delta$ residues is shown in Figure S4 the graph after the separation is shown in Figure S5. The vertex weights and two of the edge weights in this separated graph are chosen to make the unary energies in the separated case agree with the unary energies in the unseparated case.

The binary interaction energies for the revised graph are determined by solving a system of equations with the edge weights as variables. One possible solution is shown in Figure S6, obtained by solving the following system of equations:

$$
\begin{aligned}
E + I + H &= E_{HA}(\delta, 0), \quad & E + G + J &= E_{HA}(\delta, 1), \\
B + D + K &= E_{HA}(\epsilon, 0), \quad & B + C + L &= E_{HA}(\epsilon, 1), \\
H + K &= E_{HA}(\delta\epsilon, 0), \quad & G + L &= E_{HA}(\delta\epsilon, 1)
\end{aligned}
$$

This set of equations is under-determined: there are 10 variables with only 6 equations. To resolve this degeneracy, four of the variables can be arbitrarily set to zero. We chose $B = D = E = J = 0$.

The analysis for two interacting HIS residues follows the same process, although with more equations and variables (edge weights). We skip the detailed derivation and simply provide the original energy graph in Figure S7 and the new one with both HIS residues split in Figure S8. Notice that interaction (edge weights) between $\delta$ and $\epsilon$ originating from the same HIS residue are consistent between Figures S6 and S8.

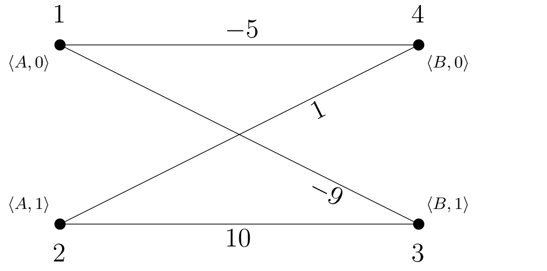


(a) Original energy graph

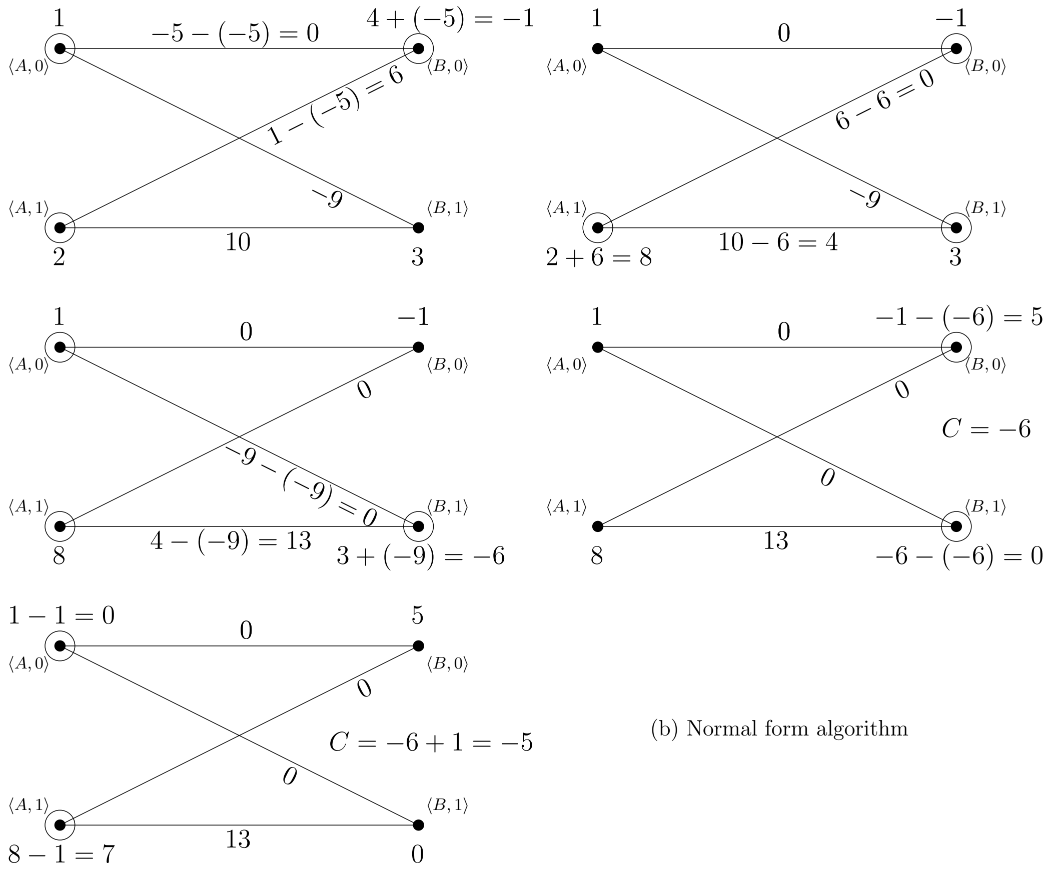


(b) Normal form algorithm

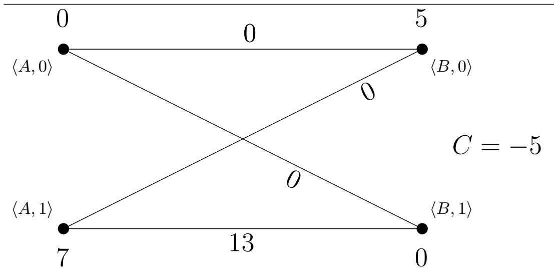


(c) Normal form energy graph

Figure S3: Illustration of the graph normal form procedure.

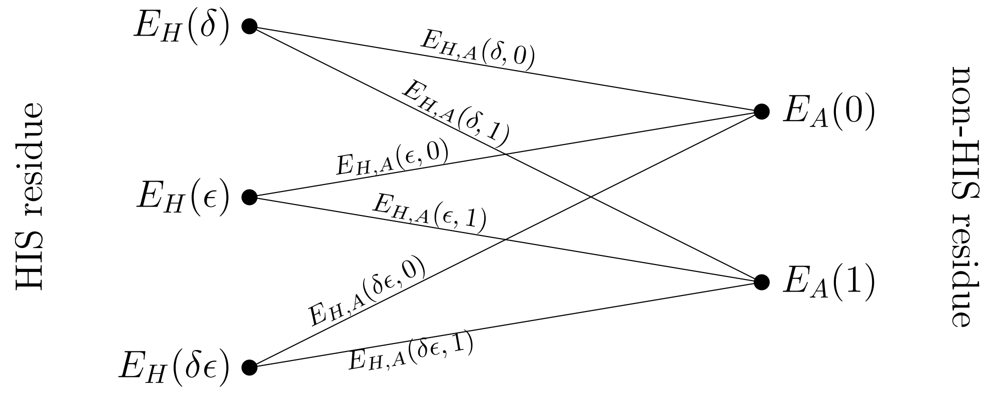


Figure S4: Energy graph for HIS with a non-HIS residue, $A$, before splitting HIS into $\text{HIS}_\epsilon$ and $\text{HIS}_\delta$.

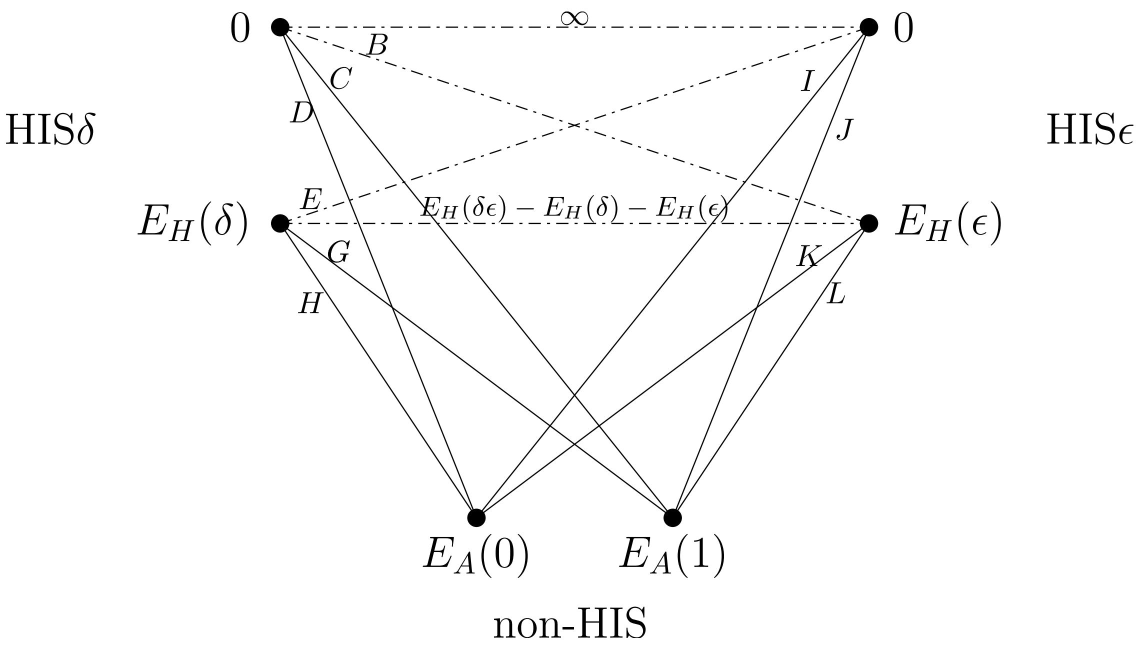


Figure S5: Energy graph for HIS with a non-HIS residue, $A$, after splitting HIS into $\text{HIS}_\epsilon$ and $\text{HIS}_\delta$. Most edge weights are variables, we solve a system equations to find the correct edge weights. The dash-dot lines represent edges, or interactions, between the two artificial HIS residues, $\text{HIS}_\epsilon$ and $\text{HIS}_\epsilon$, that originate from the same real HIS residue.

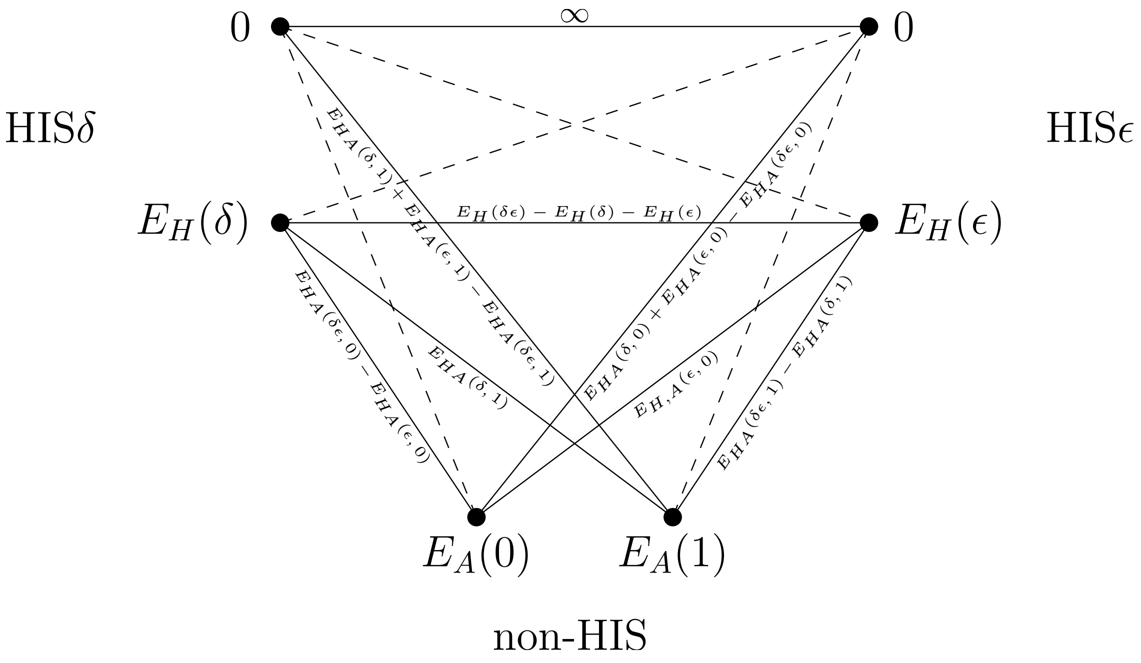


Figure S6: Energy graph for HIS with a non-HIS residue, $A$, after splitting HIS into $\text{HIS}_\epsilon$ and $\text{HIS}_\delta$. Dashed lines represent edges with weight zero.

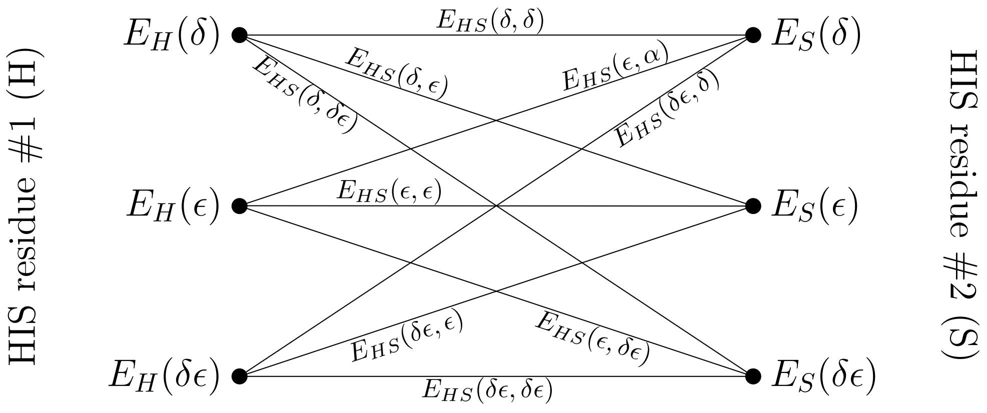


Figure S7: Energy graph for interaction between two HIS residues before splitting both into two residues.

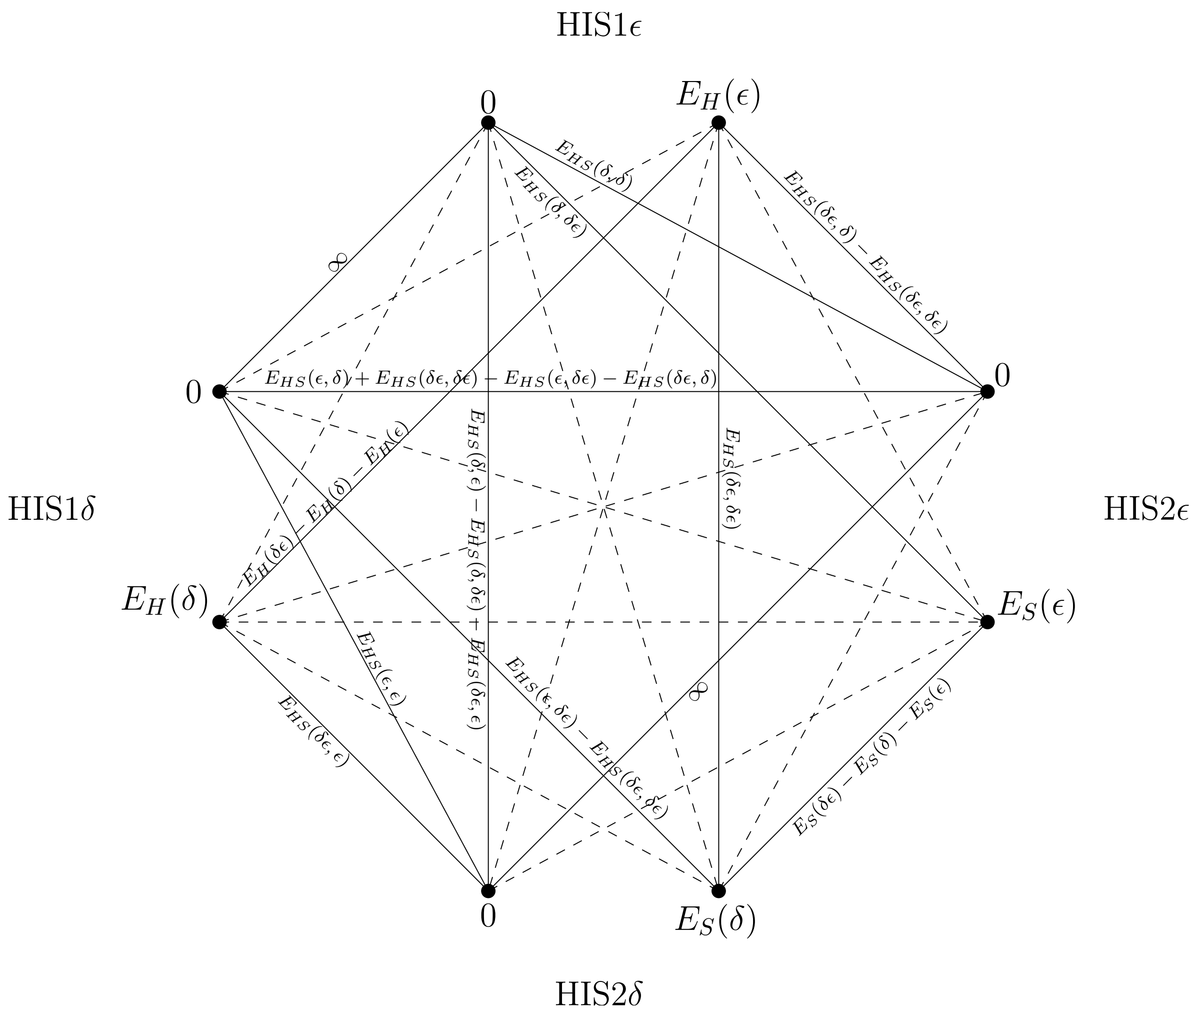


Figure S8: Energy graph for interaction between two HIS residues after splitting both. Dashed lines indicate edge weight zero.

# Titration state optimization through graph cuts

The normal form energy graph is transformed into an energy flow network using a procedure which guarantees that the minimum cut in the network will equal the minimum energy of the protein titration system. This minimum cut will also define the titration state of the minimum energy configuration. For each amino acid, $i$, we put two vertices, $v_i, \hat{v}_i$, into the vertex set for our network, where $v_i$ represents the amino acid $i$ in its deprotonated state and $\hat{v}_i$ represents amino acid $i$ in its protonated state. We also include a source and sink, $s$ and $t$, so that the complete set of vertices is $V = \{v_i, \hat{v}_i\}_{i=1}^{N} \cup \{s, t\}$. Table S1 shows how the vertex and edge weights in the normal form graph translate into edge capacities in the flow network.[6] If any pairwise or unary energy value happens to be zero after the normal form translation, the edges associated with that energy value are not included in the flow network since, according to Table S1, they would have weight zero if included. For graphical representations of each of these edges in the network, see Figure S9, Figure S10, and Figure S11. Figure S12 illustrates the transformation of the example normal form energy graph into its corresponding flow network.

Note that, after these transformation processes, the edge weights still represent energy values but are no longer interaction energies between the protonation states represented by the vertices in the edge. For example, consider the edge $[A, \hat{B}]$, where $A$ is deprotonated and $B$ is protonated; notice from Table S1, that this edge in the transformed graph has weight $\frac{1}{2}E_{AB}(0,0)$ rather than the original $\frac{1}{2}E_{AB}(0,1)$ on this edge.

Table S1: Illustration of how the vertex and edge weights in the normal form graph translate into edge capacities in the flow network.

| Capacity | $\frac{1}{2}E_i(1)$ | $\frac{1}{2}E_i(0)$ | $\frac{1}{2}E_{ij}(0,0)$ | $\frac{1}{2}E_{ij}(1,0)$ | $\frac{1}{2}E_{ij}(0,1)$ | $\frac{1}{2}E_{ij}(1,1)$ |
|---|---|---|---|---|---|---|
| Edge | $[s, v_i]$ | $[s, \hat{v}_i]$ | $[v_i, \hat{v}_j]$ | $[\hat{v}_i, \hat{v}_j]$ | $[v_i, v_j]$ | $[\hat{v}_i, v_j]$ |
| | $[\hat{v}_i, t]$ | $[v_i, t]$ | $[v_j, \hat{v}_i]$ | $[v_j, v_i]$ | $[\hat{v}_j, \hat{v}_i]$ | $[\hat{v}_j, v_i]$ |

Recall that the energy of a protonation state can be determined by choosing the vertices

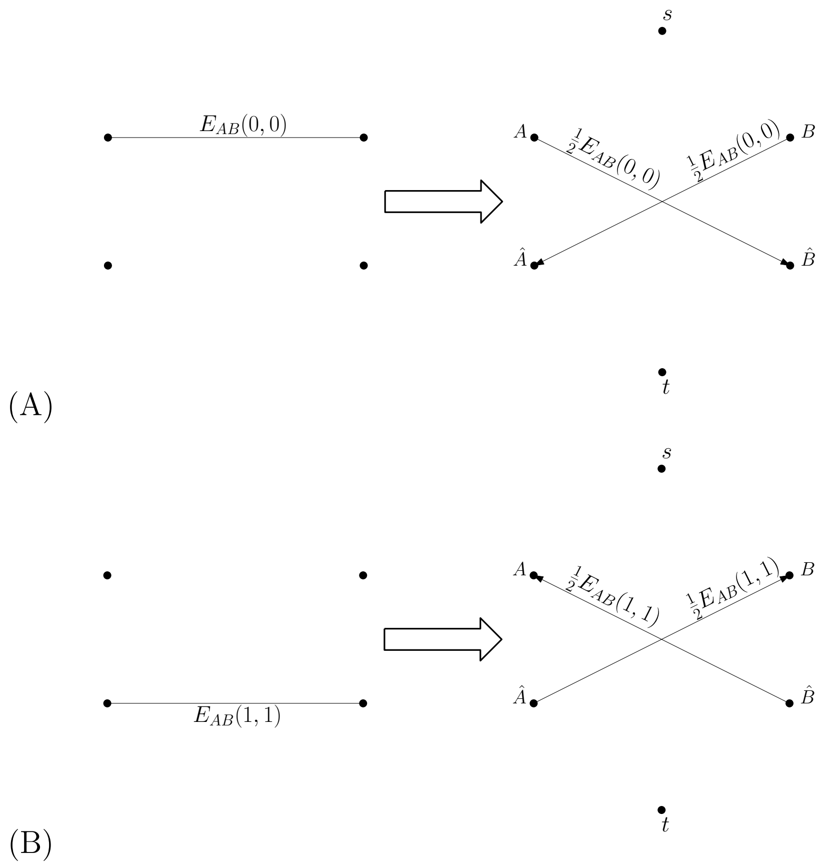


Figure S9: (A) Directed edges in the flow network corresponding to $E_{ij}(0,0)$. (B) Directed edges in the flow network corresponding to $E_{ij}(1,1)$

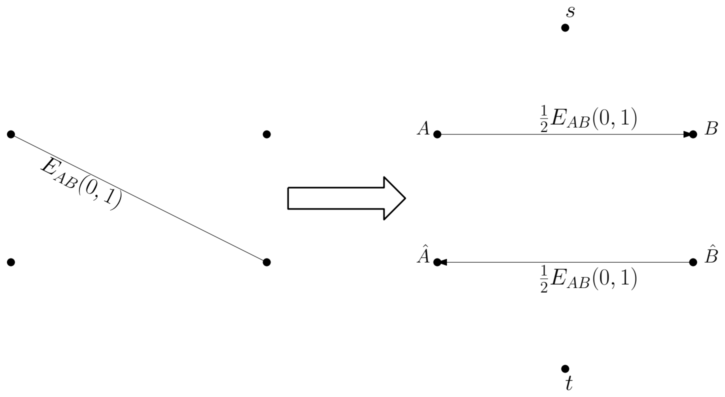


(A)

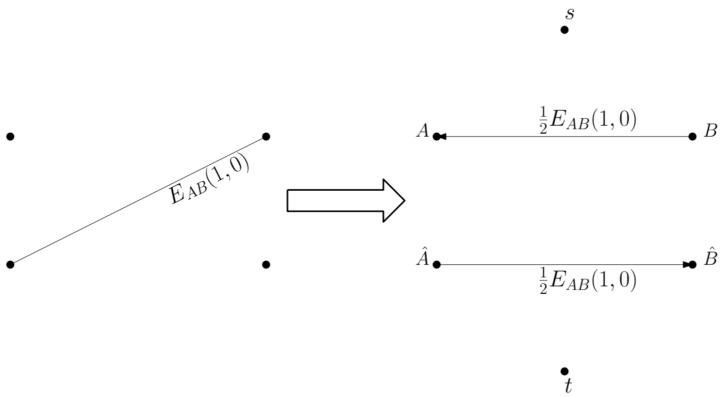


(B)

Figure S10: (A) Directed edges in the flow network corresponding to $E_{ij}(0,1)$. (B) Directed edges in the flow network corresponding to $E_{ij}(1,0)$.

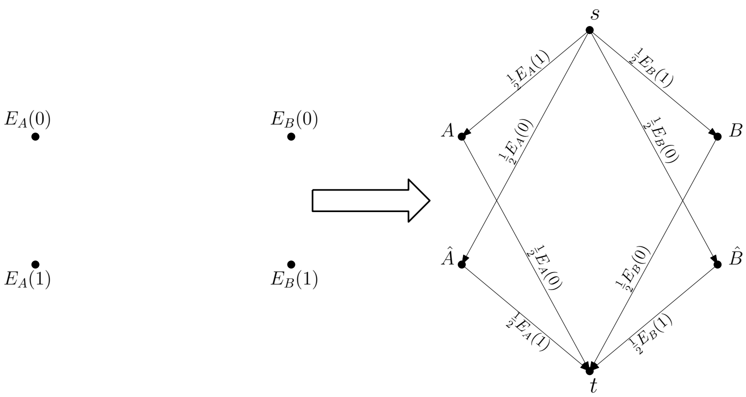


Figure S11: Directed edges in the flow network corresponding to the unary energies.

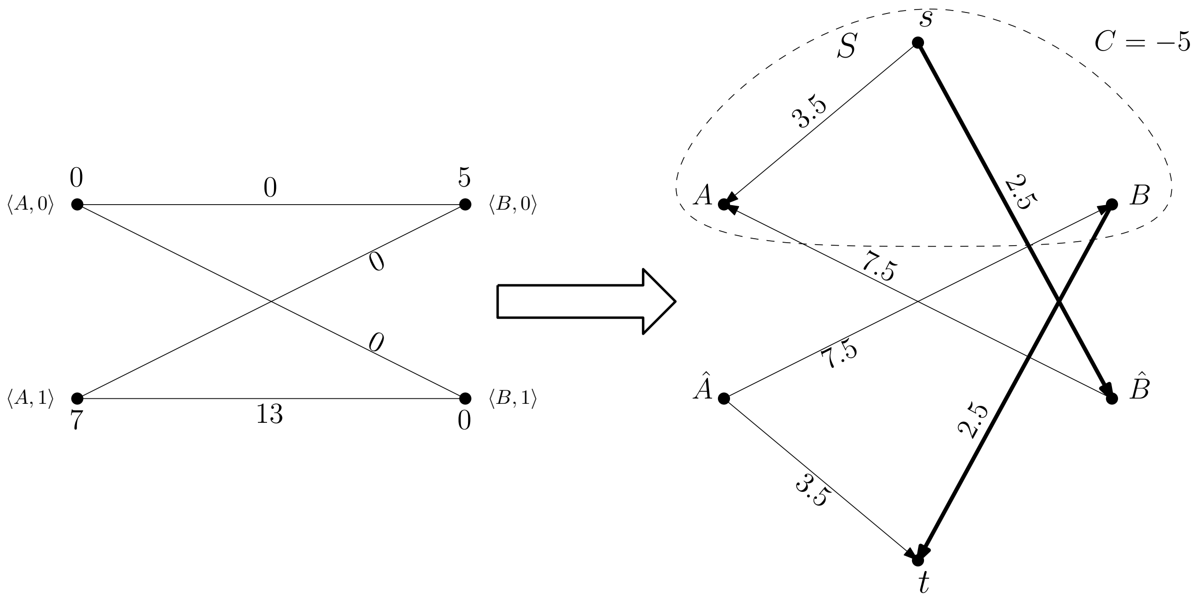


Figure S12: Flow network created from example normal form output in Figure S3. The $S$ set for the cut is indicated by the dashed line.

in the energy graph corresponding to that particular protonation state, discarding all other vertices (and corresponding edges), and taking the sum of the edge and vertex weights that remain. This selection can also be represented through a graph cut. Recall that all vertices $\{v_i\}_{i=1}^N$ correspond to the deprotonated states of the amino acids and vertices $\{\hat{v}_i\}_{i=1}^N$ correspond to the protonated states. We can form a cut from a known protonation state by letting $S$ contain $s$ along with all vertices corresponding to the correct protonation state of each residue. Then $T$ contains $t$ and all other vertices. Given the capacities in Table S1 it can be shown that the cut value associated with this cut, plus the global constant from the normal form, is exactly the energy of the associated state of the system.[6] Therefore, give a cut, $S, T$, the vertices assigned to the $S$ cut set are used to label the amino acids while the $T$ cut set contains the complement (remainder) of these states.

In the example from Figure S12, there are four possible protonation states which makes it straightforward to check that the cut value provides the correct protonation state energy. For example, if both $A$ and $B$ are deprotonated, then the energies for these states can be

obtained from the normal form (left side of Figure S12) through the following procedure: discard vertices $\langle A, 1\rangle$ and $\langle B, 1\rangle$ and all associated edges and sum the remaining edge and vertex weights along with the normal-form constant to get the energy of the system:

$$g(\langle A, 0\rangle) + g(\langle B, 0\rangle) + w(\langle A, 0\rangle, \langle B, 0\rangle) + c = 0 + 5 + 0 - 5 = 0.$$

The corresponding flow network (right side of Figure S12) can also be used to calculate the total energy: the cut for both $A$ and $B$ deprotonated is $S = \{s, A, B\}$, $T = \{t, \hat{A}, \hat{B}\}$, so edges going from $S$ to $T$ are $[s, \hat{B}]$ and $[B, t]$ (the heavier edges in Figure S12) and their capacities summed, together with the normal form constant for a total cut value of $2.5 + 2.5 - 5 = 0$. Table S2 illustrates similar calculations for each of the four possible titration states of this example system.

Table S2: The energy from normal form column is calculated using the graph in the supporting information Figure S3. Vertices (and corresponding edges) are removed if they are not in the given protonation state, as described in the text. For example, for the value in the third row, we remove vertices $\langle A, 0\rangle$ and $\langle B, 1\rangle$. Then the remaining edge and vertex weights are summed ($g(\langle A, 1\rangle) + g(\langle B, 0\rangle) + w(\langle A, 1\rangle, \langle B, 0\rangle) = 7 + 5 + 0$). Finally, the universal constant (-5) is added to the result.

| $A$ | $B$ | $S$ | $T$ | energy from normal form | cut value + constant |
|---|---|---|---|---|---|
| deprot | deprot | $\{s, A, B\}$ | $\{t, \hat{A}, \hat{B}\}$ | 5-5=0 | 2.5+2.5-5=0 |
| deprot | prot | $\{s, A, \hat{B}\}$ | $\{t, \hat{A}, B\}$ | 0-5=-5 | 0-5=-5 |
| prot | deprot | $\{s, \hat{A}, B\}$ | $\{t, A, \hat{B}\}$ | 7+5-5=7 | 3.5+3.5+2.5+2.5-5=7 |
| prot | prot | $\{s, \hat{A}, \hat{B}\}$ | $\{t, A, B\}$ | 7+13-5=15 | 3.5+3.5+7.5+7.5-5=15 |

Additional requirements are needed to ensure that the minimum cut in the network yields the minimum energy configuration. In a 2004 paper, Kolmogorov and Zabih[7] proved that if $E$ is a function of $N$ binary variables of the form

$$E(x_1, \ldots, x_N) = \sum_i E_i(x_i) + \sum_{i<j} E_{ij}(x_i, x_j)$$

and all $E_{ij}$ are submodular, then it is possible to find the exact minimum of $E$ in polynomial time by computing the minimum $s - t$ cut on the flow network of the associated graph. Protein titration site interaction networks are not guaranteed to have submodular energies. However, it is still possible to use the graph-cut method to label the portion of the amino acids whose energy functions are submodular.[6] Kolmogorov and Rother[6] prove that the amino acids which are labeled via the graph cut are guaranteed to be correctly assigned; i.e., a partial assignment, $Q$, from a minimum cut in the network is associated with a global minimum protonation state assignment, $P \in \mathcal{P}$, with the property that $Q_i = P_i$ for all amino acids that were assigned in $Q$.[6] The remaining amino acids must be assigned by some other optimization method (e.g., Monte Carlo or brute force) on only the unassigned amino acids.

## Data analysis

An iPython notebook accompanies this paper with all of the code used to perform data analysis and generate figures. One additional comparison not presented in the main manuscript (but available in the iPython notebook) is shown in Figure S13. This figure compares the p$K_a$ *shifts* for the two methods discussed in this paper. A p$K_a$ shift is defined as the difference between the observed p$K_a$ and the p$K_a$ value for a model compound.

The Python code for the graph-cut algorithm is also provided as supporting information.

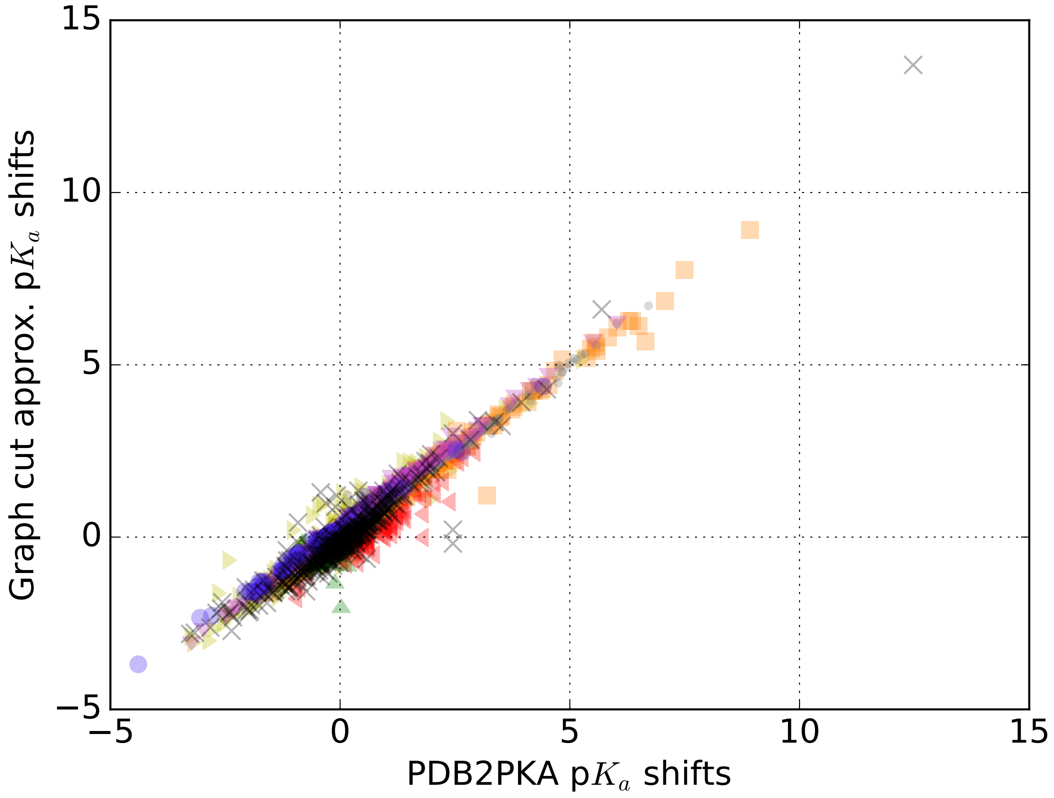


Figure S13: Comparison of p$K_a$ values calculated with the graph-cut method and with PDB2PKA. ○: arginine, □: aspartate, +: C-terminus, ×: glutamate, ∗: HIS$_\epsilon$, ⋄: HIS$_\delta$, △: lysine, ▽: N-terminus, ◁: tyrosine.

## References


(1) Diestel, R. *Graph Theory*, 3rd ed.; Springer-Verlag: Berlin Heidelberg, 2006.

(2) Ford, L. R.; Fulkerson, D. R. Maximal Flow Through a Network. *Canad. J. Math* **1956**, *8*, 399–404.

(3) Edmonds, J.; Karp, R. M. Theoretical Improvements in Algorithmic Efficiency for Network Flow Problems. *J. ACM* **1972**, *19*, 248–264.

(4) Goldberg, A. V.; Tarjan, R. E. A New Approach to the Maximum-flow Problem. *J. ACM* **1988**, *35*, 921–940.

(5) Dinic, E. Algorithm for Solution of a Problem of Maximum Flow in a Network with Power Estimation. *Soviet Math Doklady* **1970**, *11*, 1277–1280.

(6) Kolmogorov, V.; Rother, C. Minimizing Nonsubmodular Functions with Graph Cuts–A Review. *IEEE Trans. Pattern Anal. Mach. Intell.* **2007**, *29*, 1274–1279.

(7) Kolmogorov, V.; Zabih, R. What Energy Functions Can Be Minimized via Graph Cuts? *IEEE Trans. Pattern Anal. Mach. Intell.* **2004**, *26*, 147–159.
